# Supplementary material for: SkillVerse : Assessing and Enhancing LLMs with Tree Evaluation
Source: arXiv:2506.00319 source file (2025-05-31)
Supplement: Supplementary file 1 [file Report_appendix_table_2.pdf]

| High-Level Summary | Detailed description | Gemini-1.5-pro | Claude3.5-Sonnet | GPT-4o |
|---|---|---|---|---|
| **Write functional and specific-purpose code, focusing on implementation and problem-solving.** | write code for visualization purpose (e.g., scattered plot, bar chart) | 79.49% | 85.53% | 76.83% |
| | implement a feature or write code for game development (e.g., terrain generation, sprite editor) | 71.25% | 69.03% | 74.04% |
| | create or use AI/ML model/chatbot | 87.61% | 94.56% | 90.70% |
| | write SQL queries,containing specific techniques like CTEs, joins, window functions | 84.92% | 89.92% | 85.42% |
| | improve code quality (organization, efficiency, conciseness, functionality) | 62.51% | 58.81% | 70.44% |
| | comment on code quality (efficiency, readability) | 90.93% | 84.87% | 92.44% |
| | translate into first-order logic (FOL) and conjunctive normal form (CNF), | 83.85% | 78.09% | 80.44% |
| | write test cases, handling edge cases and generating the expected output | 88.99% | 97.26% | 93.86% |
| | provide detailed instructions for package installation, configuration, and setup | 96.31% | 89.28% | 91.83% |
| | write code for games/chess/elo, create card decks, solve rubiks cube | 76.79% | 73.57% | 80.78% |
| | write code or script for shell commands (file operations, automation, configuration) | 80.40% | 90.11% | 96.43% |
| | write code or function about network, stack, TCP, IP address | 74.99% | 65.23% | 70.44% |
| | Fixing bugs or troubleshooting | 86.14% | 77.92% | 94.48% |
| | write code for data processing (e.g., scrape data, convert/generate files, save files, extract content) | 79.78% | 85.14% | 86.43% |
| **Compose clear and comprehensive explanations for algorithms** | provide explanations of algorithms including aspects like steps, examples, details, and target audiences | 96.97% | 90.63% | 89.54% |
| | use examples (analogy, specific, real-world, illustrative) | 89.18% | 62.06% | 81.98% |
| | compare (pros/cons of) methods/strategies/options | 93.90% | 82.99% | 89.55% |
| | provide explanation (sentiment analysis, chatbot, LLM, Langchain, AutoGen) | 88.05% | 88.55% | 91.07% |
| | complexity analysis for algorithm | 86.93% | 87.89% | 82.83% |
| | provide helpful, correct and relevant suggestions and advice | 100.00% | 97.96% | 98.15% |
| | write documentation including comments and docstrings | 94.87% | 90.70% | 83.86% |
| **Provide mathematical analysis, calculations, or proofs.** | provide or write mathematical proofs | 62.00% | 75.73% | 83.77% |
| | calculate financial terms (interest rate, future value, present value, profit/loss, etc) or analyze (options, hedging, market behavior, etc) | 79.56% | 75.63% | 82.63% |
| | solve a (math, physics) problem | 82.35% | 88.25% | 78.46% |
| | perform calculation or derive formula | 77.42% | 70.25% | 75.46% |
| **Create and analyze technical content with practical details.** | create game related content like character sheet or game session outline | 89.20% | 70.74% | 86.51% |
| | analyze and advise on security vulnerabilities and best practices | 89.20% | 79.41% | 85.68% |
| | write music-related items (song, melody, chord progression) using formats like ABC notation and MIDI | 85.73% | 81.59% | 71.26% |
| | provide detailed business analysis like strategy, model, SWOT, market, and finance | 92.20% | 96.60% | 91.86% |
| | design on a topic like software, schema, or engineering process | 87.29% | 85.19% | 80.65% |
| | debate or evaluate arguments | 90.90% | 69.11% | 74.95% |

| High-Level Summary | Detailed description | Gemini-1.5-pro | Claude3.5-Sonnet | GPT-4o |
|---|---|---|---|---|
| **Develop, evaluate, and refine diverse content (creative, educational)** | provide comprehensive recipe (ingredient, flavor, nutrition, instruction) | 93.29% | 92.97% | 85.72% |
| | create a structured and well-organized curriculum or outline for a course (covering topics, levels, titles) | 95.22% | 97.31% | 88.28% |
| | write creative content like story, script, lyrics, article | 79.55% | 81.85% | 70.26% |
| | translate or analyze (grammar, meaning, usage) of language and write in a specific style (tone, format) | 84.50% | 86.47% | 82.01% |
| | create a detailed training plan with time estimates and specific workouts | 80.48% | 76.45% | 66.69% |
| | categorize, extract, and identify entities, relationships, from long context | 78.81% | 82.65% | 75.01% |
| **Focus on clarity, conciseness, and formatting in writing.** | structure text using headings, (numbered) bullet points, and bolding | 91.65% | 80.00% | 88.72% |
| | write in a clear, well-organized, easy to understand, and readable format (e.g., formatting, structure, clarity) | 92.37% | 89.20% | 88.72% |
| | provide relevant explanation | 96.64% | 90.01% | 95.81% |
| | be concise and to the point (instead of overly verbose, repetitive) | 95.21% | 100.00% | 91.32% |
| | write concisely, balancing the level of detail (using examples, visual aids) | 84.85% | 72.74% | 91.50% |
| **Understand and address user intent with clear, structured responses.** | address vague requests and identify the user's actual ntent | 63.18% | 63.18% | 83.68% |
| | understand and fulfill the prompt, addressing requirements, instructions, and questions | 91.53% | 89.50% | 89.99% |
| | provide help on ethical related issues | 97.81% | 92.74% | 97.32% |
| | not refuse too many requests due to ethical concerns | 63.34% | 83.77% | 87.26% |
| | provide resources (links, references) | 72.02% | 69.39% | 78.28% |
| | provide truthful, relevant, accurate, and factual information | 77.38% | 80.97% | 80.52% |
| | write about comprehensive details (scope, limitations, potential issues) | 89.29% | 83.78% | 87.42% |
| | | | | |
| | | | | |
| | | | | |
| | | 81.71% | 81.38% | 84.61% |
